# Supplementary material for: JUNO: Optimizing High-Dimensional Approximate Nearest Neighbour Search with Sparsity-Aware Algorithm and Ray-Tracing Core Mapping
Source: arXiv:2312.01712 source file (2023-12-04)
Supplement: Supplementary file 1 [file supplemental.tex]

\section*{Supplemental Materials}
\thispagestyle{empty}
We provide several supplemental materials of our main text for higher readibility. 
\paragraph{Pseudocode of \proj{} End-to-end Pipeline.}
Following pseudocode describe the \proj{} end-to-end search pipeline consists of proposed components in the main text, and is an identical but formal description of \Fig{fig-Overview} in the main text.
\begin{algorithm}[h]
	\caption{\proj{} end to end.}
	\label{Algo-e2e}
	\small
    \textbf{Input:} $points[N][D]$, $queries[Q][D]$\\
    \textbf{Input:} $K$, $M=2$, $E$, $C$, $nprobs$\\
    \textbf{Output:} $neighbours\lbrack Q\rbrack\lbrack K\rbrack$
	\begin{algorithmic}[1]
		\Function {JUNO}{$points$, $queries$, $K$, $M$, $E$, $C$, $Q$, $nprobs$}
        \State{$I\leftarrow BuildRTScene(points, M, E, C, r)$}
        \State{$q\_select\_clusters\lbrack Q\rbrack\leftarrow\lbrack~\rbrack$}
        \State{\textbf{// Filtering}}
        \For{ $q$\textbf{ in }$queries$}
            \State{$I.centroids.sort(\lambda~x:L2(x,q)/IP(x,q))$}
            \State{$q\_select\_clusters[q]\leftarrow centroids[0:nprobs]$}
        \EndFor
        \State{\textbf{// Threshold based selective L2-LUT construction}}
        \State{$LUT\leftarrow L2\_LUT(queries,I,q\_select\_clusters)$}
        \State{\textbf{// Distance calculation of interested search points}}
        \For{$q$\textbf{ in }$queries$}
            \State{$result[q]\leftarrow DistCalc(q, LUT[q], I.Map).Top(K)$}
        \EndFor
        \State{\textbf{return }$result$}
		\EndFunction
	\end{algorithmic}
\end{algorithm}
\newpage
\paragraph{Pseudocode of Distance Calculation.}
Following pseudocode describe the implementation of distance calculation with selective L2-LUT in details, and is an identical but formal description of last paragraph in \Sec{sec:OnlinePhase}.
\begin{algorithm}[h]
    \small
        \caption{Construct L2-LUT with the RT core and conduct distance calculation for interested search points.}
        \label{Algo-DistCalc}
        % Move to supply
        \textbf{Input:} $query$, $LUT$, $Map$\\
        \textbf{Output:} $neighbors$
        \begin{algorithmic}[1]
            \Function {DistCalc}{$query$, $LUT$, $Map$}
            \State{$neighbors\leftarrow \lbrace id: tot\_d\rbrace$}
            \For{$c\in[0,nprobs), s\in[0,\frac{D}{M})$}
                \State{$item\leftarrow LUT[c][s]$}
                \State{$e, d\leftarrow item.entry, item.distance$}
                \For{$p$\textbf{ in }$neighbors$}
                    \State{$p.tot\_d$ += $d~if~p.id\in Map[c][s][e]$}
                \EndFor
            \EndFor
            \EndFunction
        \end{algorithmic}
    \end{algorithm}
  
\paragraph{Latency Results of \proj{} on SIFT1M and DEEP1M.}
We also provide latency result of \proj{}, as shown in following figures.
\begin{figure}[h]
      \centering
          \includegraphics[width=0.49\linewidth]{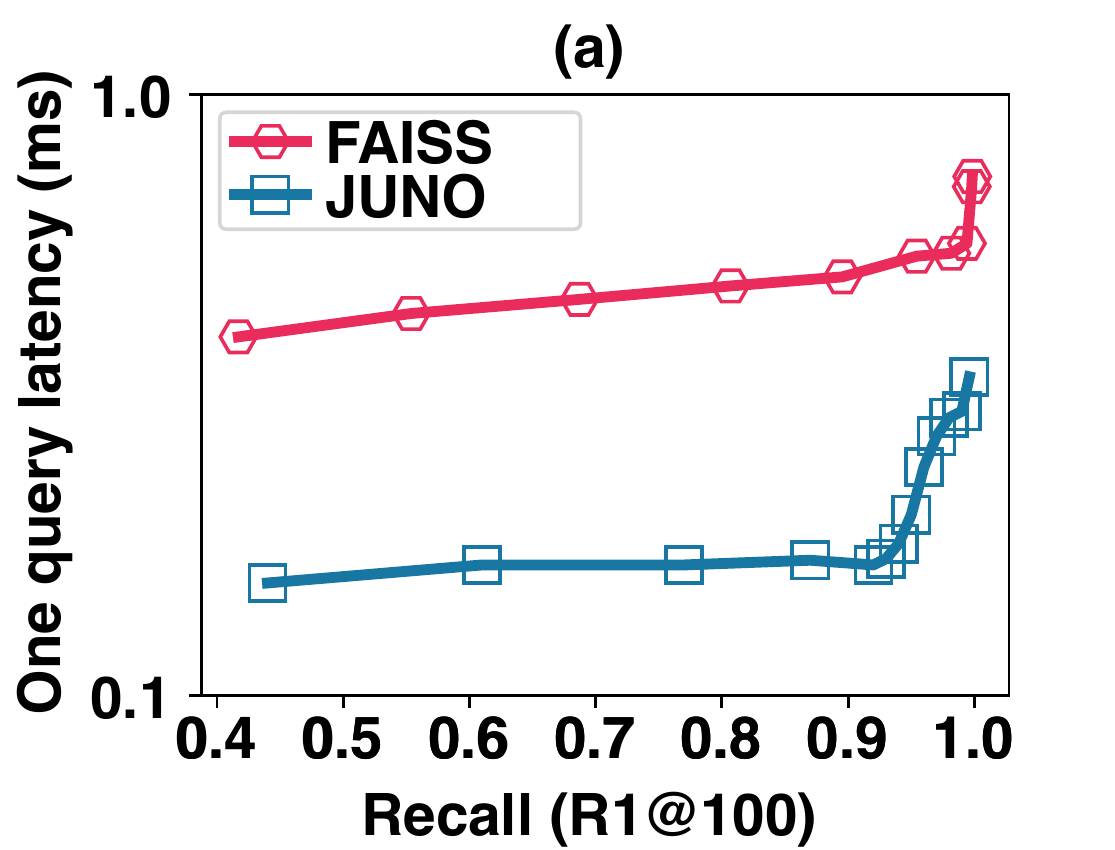}
        \includegraphics[width=0.49\linewidth]{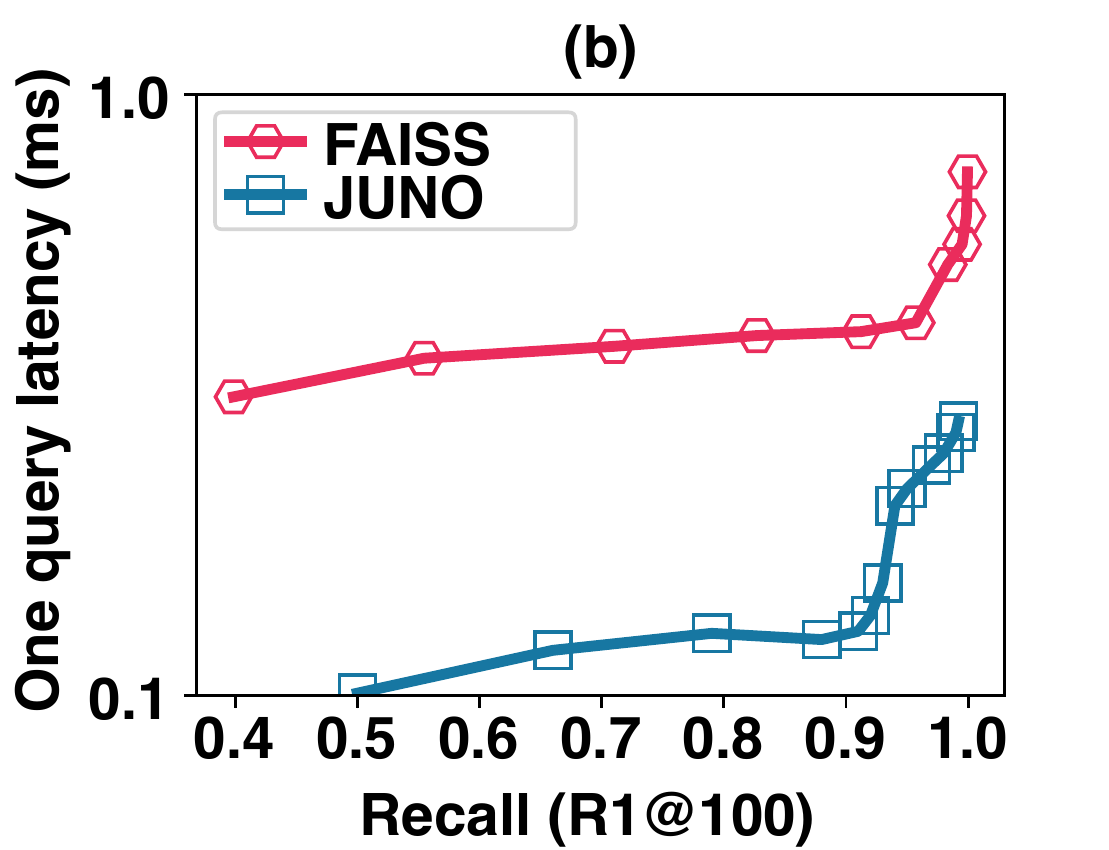}
      \caption{Latency of searcing a single query of SIFT1M (a) and DEEP1M (b), respectively. We choose the lowest latency of FAISS with different product quantization configurations.}
      \label{fig-Latency} 
  \end{figure}
